# Supplementary material for: Coupled Time-lapse Full Waveform Inversion for Subsurface Flow Problems using Intrusive Automatic Differentiation
Source: arXiv:1912.07552 source file (2020-05-05)
Supplement: Supplementary file 1 [file si_main.pdf]

# Supporting Information for "Coupled Time-lapse Full Waveform Inversion for Subsurface Flow Problems using Intrusive Automatic Differentiation"

Dongzhuo Li[1*], Kailai Xu[2 *], Jerry M. Harris[1,2], Eric Darve[2,3]

[1]Department of Geophysics, Stanford University, Stanford, CA, 94305

[2]Institute for Computational and Mathematical Engineering, Stanford University, Stanford, CA, 94305

[3]Mechanical Engineering, Stanford University, Stanford, CA, 94305

## Contents of this file

1. Text S1 to S8
2. Figures S1 to S5

## SI 1. More Details on the Physics Models

### SI 1.1. The Flow Physics Model

To solve the flow equations, we define the potentials of each phase as

$$\Psi_i = P_i - \rho_i g Z, \quad i = 1, 2, \tag{S1}$$

as well as the capillary potential

$$\Psi_c = P_c - (\rho_1 - \rho_2) g Z. \tag{S2}$$

---

*Both authors contributed equally to this work.

We ignore the capillary pressure but retain the gravity term, hence $\Psi_c = -(\rho_1 - \rho_2)gZ$.

With the assumption of incompressibility and immiscibility of the fluids, and Eq. (10) and Eq. (11), we can obtain the following potential equation,

$$-\nabla \cdot (m_t K \nabla \Psi_2) = \nabla \cdot (m_1 K \nabla \Psi_c) + q, \tag{S3}$$

where $q = q_1 + q_2$, where $q_1$ and $q_2$ are injection/production rate of fluid phase 1 and 2, respectively. With $\Psi_\alpha$, we can compute $v_\alpha$, and obtain the saturation equation as,

$$\phi \frac{\partial S_2}{\partial t} - \nabla \cdot (m_2 K \nabla \Psi_2) = q_2 \tag{S4}$$

Hence, we have decoupled the original system of equations into two sub-equations and can solve them alternatively. Note that if we keep the production rate of fluid 1 as $q_1$ and if the capillary pressure is zero, the injection/production rate of fluid 2 is $q_2(\mathbf{x}, t) + q_1(\mathbf{x}, t)\frac{m_2(\mathbf{x},t)}{m_1(\mathbf{x},t)}$, which means at the production well fluid 2 is also produced in proportion to fluid 1.

We adopt the no-flow boundary condition which reads as,

$$\mathbf{v}_i \cdot \mathbf{n} = 0, i = 1, 2, \tag{S5}$$

where $\mathbf{n}$ is the outward unit normal vector on the boundary. To apply this condition to our system, we define another two velocities as,

$$\mathbf{v}_t = -m_t K \nabla \Psi_2 \tag{S6}$$

$$\mathbf{v}_c = -m_1 \nabla \Psi_c. \tag{S7}$$

One can verify that $\mathbf{v}_1 + \mathbf{v}_2 = \mathbf{v}_t + \mathbf{v}_c$, and $\mathbf{v}_2 = m_2 \mathbf{v}_t$, from which we deduce that

$$\mathbf{v}_t \cdot \mathbf{n} = 0, \text{ and } \mathbf{v}_c \cdot \mathbf{n} = 0. \tag{S8}$$

Therefore, for the potential equation, the boundary conditions are

$$\mathbf{n} \cdot \nabla \Psi_2 = 0, \text{ and } \mathbf{n} \cdot \nabla \Psi_c = 0. \tag{S9}$$

It is insufficient to solve the potential equation (a Poisson's equation) only with the above Neumann boundary conditions; thus, we prescribe a Dirichlet boundary condition by forcing the potential to be a specific value at one point of the boundary.

## SI 1.2. Rock Physics Models

### SI 1.2.1. Patchy Saturation Model

If we have an estimation of P- and S-wave velocities and rock density before injection ($C_{p1}$, $C_{s1}$ and $\rho_{r1}$), we can compute the bulk modulus $B_{r1}$ and shear modulus $\mu$ for rock fully saturated with fluid 1:

$$B_{r1} = \rho_{r1} \left( C_{p1}^2 - \frac{4}{3} C_{s1}^2 \right), \tag{S10}$$

and

$$\mu = \rho_{r1} C_{s1}^2. \tag{S11}$$

The patchy saturation model is suitable for the situation in which different fluids form isolated patches with a scale much larger than the pore space. The rock is stiffer than the case where fluids are well mixed in pore spaces. In the patchy saturation model, we first compute the bulk modulus of rock fully saturated with fluid 2 ($B_{r2}$) by solving

$$\frac{B_{r2}}{B_o - B_{r2}} = \frac{B_{r1}}{B_o - B_{r1}} - \frac{B_{f1}}{\phi \left( B_o - B_{f1} \right)} + \frac{B_{f2}}{\phi \left( B_o - B_{f2} \right)}. \tag{S12}$$

Then, the bulk modulus of partially saturated rock as a function of saturation of fluid 2 is

$$B_r(S_2) = \left[ (1 - S_2) \left( B_{r1} + \frac{4}{3}\mu \right)^{-1} + S_2 \left( B_{r2} + \frac{4}{3}\mu \right)^{-1} \right]^{-1} - \frac{4}{3}\mu. \tag{S13}$$

Since the shear modulus of fluids is zero, we assume that the rock shear modulus does not change with $S_2$ replacing $S_1$. Therefore, the first Lamé parameter $\lambda$ is

$$\lambda(S_2) = B(S_2) - \frac{2}{3}\mu. \tag{S14}$$

To calculate density, we note that the densities of rock fully saturated with fluid 1 ($\rho_{r1}$) and with fluid 2 ($\rho_{r2}$) have the following relationship

$$\begin{cases} \rho_{r1} = \rho_o(1-\phi) + \phi\rho_1 \\ \rho_r(S_2) = \rho_o(1-\phi) + \phi\left[(1-S_2)\,\rho_1 + S_2\rho_2\right], \end{cases} \tag{S15}$$

where $S_2$ is the saturation of fluid 2, $\rho_o$ denotes the density of rock grains, $\rho_i, (i = 1, 2)$ are the density of fluid 1 and 2, respectively. Thus, we obtain the rock density as a function of the saturation of fluid 2 as

$$\rho(S_2) = \rho_{r1} + \phi S_2(\rho_2 - \rho_1). \tag{S16}$$

With the elastic properties $\lambda$, $\mu$ and $\rho$, we compute the elastic wavefield with Eq. (17).

### SI 1.2.2. Gassmann's Model with Brie's Fluid Mixing Equation

Gassmann's model with Brie's fluid mixing equation (Brie et al., 1995) is an empirical relationship that is able to describe the situation where two types of fluids are not completely segregated in patches. In Gassmann's model, the first step is to compute the bulk modulus of mixed fluid $K_{f\_\mathrm{mix}}$:

$$B_{f\_\mathrm{mix}} = (B_{f1} - B_{f2})(1 - S_2)^e + B_{f2}, \tag{S17}$$

where $e$ is the Brie model coefficient. The second step is to use Gassmann's equation to compute the bulk modulus of the rock partially saturated with fluid 2 $B_r(S_2)$:

$$\frac{B_r}{B_o - B_r} = \frac{B_{r1}}{B_o - B_{r1}} - \frac{B_{f1}}{\phi\,(B_o - B_{f1})} + \frac{B_{f\_\mathrm{mix}}}{\phi\,(B_o - B_{f\_\mathrm{mix}})}. \tag{S18}$$

If $e = 1$, it is close to the patch saturation model, and if $e$ is substantially large the model behaves like the Gassmann model with the Reuss average of fluids (Mavko et al., 2009). Usually, $e$ is chosen as 3. As we see in Section 4.3 that with the Gassmann's model, rock P-wave velocity drops more quickly at the beginning of $CO_2$ injection and

increases later because of the decrease in density; while in the patchy saturation model, rock P-wave velocity almost follows a straight line against $CO_2$ saturation. Although this is an empirical closure relationship, we show in Section 4.3 that it is also possible to update the coefficient $e$ simultaneously with intrinsic parameter inversion.

## SI 2. Discrete Adjoint Method

The adjoint method is an effective technique to derive gradients for large-scale PDE-constrained inverse problems, such as full-waveform inversion, history matching (Oliver & Chen, 2011; R. Li et al., 2001), 4D variational weather data assimilation (Wang et al., 2001), ocean model inversion (Marotzke et al., 1999), etc. Our inversion method is also based on the adjoint method, which we briefly introduce here.

Consider an inverse problem of the following form:

$$\begin{aligned} &\min_{\boldsymbol{\theta}} \mathcal{J}(\mathbf{u}(\boldsymbol{\theta})) \\ &\text{s.t. } \mathcal{A}\Big(\mathbf{u}(\boldsymbol{\theta}), \boldsymbol{\theta}\Big) = 0, \end{aligned} \tag{S19}$$

where $J$ is a functional of $\mathbf{u}$, which is obtained by solving a differential equation $\mathcal{A}(\mathbf{u}, \boldsymbol{\theta}) = 0$. The constraint either explicitly or implicitly establishes that $\mathbf{u}$ is a function of $\boldsymbol{\theta}$, the unknown parameter to be solved for. To solve this problem, one may use the method of Lagrange multipliers to transform this constrained problem into an unconstrained problem as

$$\min_{\boldsymbol{\theta}, \mathbf{u}} \max_{\boldsymbol{\lambda}} \mathcal{L}(\boldsymbol{\theta}, \mathbf{u}, \boldsymbol{\lambda}) = \mathcal{J}(\mathbf{u}) + \boldsymbol{\lambda}^T \mathcal{A}\Big(\mathbf{u}, \boldsymbol{\theta}\Big). \tag{S20}$$

According to the KKT condition, the necessary condition for achieving an optimum is

$$\frac{\partial \mathcal{L}}{\partial \boldsymbol{\theta}} = 0, \quad \frac{\partial \mathcal{L}}{\partial \mathbf{u}} = 0, \quad \frac{\partial \mathcal{L}}{\partial \boldsymbol{\lambda}} = 0 \tag{S21}$$

Although one may update $\boldsymbol{\theta}, \mathbf{u}$, and $\boldsymbol{\lambda}$ simultaneously using methods such as gradient descent plus dual ascent until they satisfy condition (S21), it is more common and

feasible to require that the KKT condition for both $\mathbf{u}$ and $\boldsymbol{\lambda}$ is satisfied throughout the optimization process. The latter strategy is the so-called adjoint method. In other words, we have

$$\frac{\partial \mathcal{L}}{\partial \boldsymbol{\lambda}} = \mathcal{A}(\mathbf{u}, \boldsymbol{\theta}) = 0 \tag{S22}$$

$$\frac{\partial \mathcal{L}}{\partial \mathbf{u}} = \mathcal{J}_{\mathbf{u}} + \boldsymbol{\lambda}^T \mathcal{A}_{\mathbf{u}} = 0. \tag{S23}$$

The first equation is just the normal PDE constraint where we solve for $\mathbf{u}$, while the second is the adjoint equation from which we can find the Lagrange multiplier or dual variable $\boldsymbol{\lambda}$ once we have obtained $\mathbf{u}$. One uses

$$\frac{\mathrm{d}\mathcal{J}}{\mathrm{d}\boldsymbol{\theta}} = \frac{\partial \mathcal{L}}{\partial \boldsymbol{\theta}} = \boldsymbol{\lambda}^T \mathcal{A}_{\boldsymbol{\theta}}, \tag{S24}$$

to calculate the gradient of the objective function to the parameter and then use gradient-based optimization methods to solve the problem. Note that the first equality of Eq. (S24) comes from the fact that we keep $\mathcal{A}(\mathbf{u}, \boldsymbol{\theta}) = 0$ as in Eq. (S22). We also point out that we adopt the discretize-then-optimize strategy. Namely, we discrete the constraint PDE first and then derive the discrete adjoint equation and gradient. It is easier to obtain a numerically exact gradient in this way.

One interesting fact deduced from Eq. (S23) is that the adjoint equation is always linear, despite that the forward equation may be nonlinear.

In Section SI 4, we demonstrate how to apply the discretized-adjoint method to the first-order elastic wave equation system with the CPML boundary condition.

## SI 3. The connection between Automatic Differentiation and the Discrete Adjoint Method

Let us consider a simplified inverse problem for slow-time processes illustrated in Fig. SI 1. The nodes are variables, and arrows indicate operations. The property $\mathbf{u}$ evolves from the initial condition $\mathbf{u}_1$ to $\mathbf{u}_4$, whose behavior is also controlled by the parameter $\boldsymbol{\theta}$. We may decompose the mapping into sequential steps such as $f_1, \cdots, f_4$. The last operator $f_4$ computes the objective function $\mathcal{J}$. Mathematically, the mappings are written as

$$\begin{aligned} \mathbf{u}_2 &= f_1(\mathbf{u}_1, \boldsymbol{\theta}) \\ \mathbf{u}_3 &= f_2(\mathbf{u}_2, \boldsymbol{\theta}) \\ \mathbf{u}_4 &= f_3(\mathbf{u}_3, \boldsymbol{\theta}) \\ \mathcal{J} &= f_4(\mathbf{u}_1, \mathbf{u}_2, \mathbf{u}_3, \mathbf{u}_4). \end{aligned} \tag{S25}$$

Then, we construct the following inverse problem,

$$\begin{aligned} &\min_{\mathbf{u}_1, \boldsymbol{\theta}} f_4(\mathbf{u}_1, \mathbf{u}_2, \mathbf{u}_3, \mathbf{u}_4), \\ &\text{s.t. } \mathbf{u}_2 = f_1(\mathbf{u}_1, \boldsymbol{\theta}), \\ &\qquad \mathbf{u}_3 = f_2(\mathbf{u}_2, \boldsymbol{\theta}), \\ &\qquad \mathbf{u}_4 = f_3(\mathbf{u}_3, \boldsymbol{\theta}). \end{aligned} \tag{S26}$$

Following the adjoint method in Section 2, we obtain the Lagrangian as

$$\mathcal{L} = f_4(\mathbf{u}_1, \mathbf{u}_2, \mathbf{u}_3, \mathbf{u}_4) + \boldsymbol{\lambda}_2^T(f_1(\mathbf{u}_1, \boldsymbol{\theta}) - \mathbf{u}_2) + \boldsymbol{\lambda}_3^T(f_2(\mathbf{u}_2, \boldsymbol{\theta}) - \mathbf{u}_3) + \boldsymbol{\lambda}_4^T(f_3(\mathbf{u}_3, \boldsymbol{\theta}) - \mathbf{u}_4) \tag{S27}$$

Taking the derivate of $\mathcal{L}$ with respect to $\mathbf{u}_i$ and $\theta$, and setting them to zero yields

$$\begin{aligned} \boldsymbol{\lambda}_4^T &= \frac{\partial f_4}{\partial \mathbf{u}_4} \\ \boldsymbol{\lambda}_3^T &= \frac{\partial f_4}{\partial \mathbf{u}_3} + \boldsymbol{\lambda}_4^T \frac{\partial f_3}{\partial \mathbf{u}_3} \\ \boldsymbol{\lambda}_2^T &= \frac{\partial f_4}{\partial \mathbf{u}_2} + \boldsymbol{\lambda}_3^T \frac{\partial f_2}{\partial \mathbf{u}_2} \\ \frac{\partial \mathcal{L}}{\partial \boldsymbol{\theta}} &= \boldsymbol{\lambda}_2^T \frac{\partial f_1}{\partial \boldsymbol{\theta}} + \boldsymbol{\lambda}_3^T \frac{\partial f_2}{\partial \boldsymbol{\theta}} + \boldsymbol{\lambda}_4^T \frac{\partial f_3}{\partial \boldsymbol{\theta}} \to 0. \end{aligned} \tag{S28}$$

We can recognize that the Lagrange multipliers or adjoint variable $\boldsymbol{\lambda}_i^T = \frac{\partial J}{\partial \mathbf{u}_i}, i = 2, 3, 4;$ that is, they are the partial derivative of the objective respect to intermediate variables. In Eqs (S28), the parent nodes collect $\boldsymbol{\lambda}_i$ from their child nodes. Equivalently, $\boldsymbol{\lambda}_i$ are "back-propagated" to the parent nodes pointing to node $i$, followed by multiplications such as $\boldsymbol{\lambda}_4^T \frac{\partial f_3}{\partial \boldsymbol{\theta}}$. This is exactly the same "back-propagation" scheme in the reverse-mode automatic differentiation, but AD is different in the programming interface, in which we only need to implement two methods for each customized operator:

1. Forward operation $f_n$: compute the output by solving a certain PDE.
2. Backward operation $b_n$: given gradient $\frac{\partial \mathcal{J}}{\partial \mathbf{u}_{n+1}}$, compute $\frac{\partial \mathcal{J}}{\partial \mathbf{u}_{n+1}} \frac{\partial f_n}{\partial \mathbf{u}_n}$ and $\frac{\partial \mathcal{J}}{\partial \mathbf{u}_{n+1}} \frac{\partial f_n}{\partial \theta}$ with the chain rule. Note that only a matrix-vector product needs to be implemented, and there should be no need to construct Jacobian matrices like $\frac{\partial f_n}{\partial \mathbf{u}_n}$ explicitly.

$$\frac{\partial \mathcal{J}}{\partial \mathbf{u}_{n+1}} \frac{\partial f_n}{\partial \mathbf{u}_n}, \quad \frac{\partial \mathcal{J}}{\partial \mathbf{u}_{n+1}} \frac{\partial f_n}{\partial \boldsymbol{\theta}} = b_n \left( \frac{\partial \mathcal{J}}{\partial \mathbf{u}_{n+1}}, \mathbf{u}_{n+1}, \mathbf{u}_n, \boldsymbol{\theta} \right) \tag{S29}$$

## SI 4. Discretization of the Wave Equation & Derivation of Its Adjoint System and Gradients

We use operator $D_z^+, D_x^+$ and $D_z^-, D_x^-$ to denote the fourth-order staggered grid finite difference operators in either $z$ axis or $x$ axis. The plus sign means that the finite difference is forward, while the minus sign means backward. For example,

$$\begin{aligned} D_z^+ c_{ij} &:= \left[ \frac{9}{8} \left( c_{i+1,j} - c_{i,j} \right) - \frac{1}{24} \left( c_{i+2,j} - c_{i-1,j} \right) \right] \frac{1}{\Delta z} \\ D_z^- c_{ij} &:= \left[ \frac{9}{8} \left( c_{i,j} - c_{i-1,j} \right) - \frac{1}{24} \left( c_{i+1,j} - c_{i-2,j} \right) \right] \frac{1}{\Delta z} \end{aligned} \tag{S30}$$

The staggered grid layout is illustrated in Figure SI 2, which features the configuration of wavefield variables and elastic parameters in the $ij$-th cell.

The discretized elastic wave equation with CPML boundary condition is

$$
\begin{aligned}
&\varphi_{zz}^{t+1} - b_z \varphi_{zz}^{t} - a_z D_z^- V_z^t = 0\\
&\varphi_{xx}^{t+1} - b_x \varphi_{xx}^{t} - a_x D_x^- V_x^t = 0\\
&S_{zz}^{t+1} - S_{zz}^{t} - (\lambda + 2\mu)\left[\frac{1}{K_z} D_z^- V_z^t + \varphi_{zz}^{t+1}\right]\Delta t - \lambda \left[\frac{1}{K_x} D_x^- V_x^t + \varphi_{xx}^{t+1}\right]\Delta t - c_z f^t \Delta t = 0\\
&S_{xx}^{t+1} - S_{xx}^{t} - \lambda \left[\frac{1}{K_z} D_z^- V_z^t + \varphi_{zz}^{t+1}\right]\Delta t - (\lambda + 2\mu)\left[\frac{1}{K_x} D_x^- V_x^t + \varphi_{xx}^{t+1}\right]\Delta t - c_x f^t \Delta t = 0\\
&\varphi_{xz}^{t+1} - b_{zh} \varphi_{xz}^{t} - a_{zh} D_z^+ V_x^t = 0\\
&\varphi_{zx}^{t+1} - b_{xh} \varphi_{zx}^{t} - a_{xh} D_x^+ V_z^t = 0\\
&S_{xz}^{t+1} - S_{xz}^{t} - \mu_{\text{ave}}\left[\frac{1}{K_{zh}} D_z^+ V_x^t + \varphi_{xz}^{t+1} + \frac{1}{K_{xh}} D_x^+ V_z^t + \varphi_{zx}^{t+1}\right]\Delta t = 0\\
&\phi_{zz\_z}^{t+1} - b_{zh} \phi_{zz\_z}^{t} - a_{zh} D_z^+ S_{zz}^{t+1} = 0\\
&\phi_{xz\_x}^{t+1} - b_{x} \phi_{xz\_x}^{t} - a_{x} D_x^- S_{xz}^{t+1} = 0\\
&V_z^{t+1} - V_z^t - \left[\frac{1}{K_{zh}} D_z^+ S_{zz}^{t+1} + \phi_{zz\_z}^{t+1} + \frac{1}{K_x} D_x^- S_{xz}^{t+1} + \phi_{xz\_x}^{t+1}\right]\frac{1}{\rho_a}\Delta t = 0\\
&\phi_{xz\_z}^{t+1} - b_{z} \phi_{xz\_z}^{t} - a_{z} D_z^- S_{xz}^{t+1} = 0\\
&\phi_{xx\_x}^{t+1} - b_{xh} \phi_{xx\_x}^{t} - a_{xh} D_x^+ S_{xx}^{t+1} = 0\\
&V_x^{t+1} - V_x^t - \left[\frac{1}{K_{z}} D_z^- S_{xz}^{t+1} + \phi_{xz\_z}^{t+1} + \frac{1}{K_{xh}} D_x^+ S_{xx}^{t+1} + \phi_{xx\_x}^{t+1}\right]\frac{1}{\rho_b}\Delta t = 0,
\end{aligned}
\tag{S31}
$$

where the space index $i, j$ is omitted for all variables for brevity. In other words, $S_{zz}^{t+1}$ is a shorthand for $S_{zz;i,j}^{t+1}$. In this system of discretized PDEs, $\varphi_{zz}, \varphi_{xx}, \varphi_{xz}, \varphi_{zx}$ are CPML memory variables for computing spatial derivatives of the particle velocities $V_z, V_x$. Similarly, $\phi_{zz\_z}, \phi_{xz\_x}, \phi_{xz\_z}, \phi_{xx\_x}$ are CPML memory variables for computing spatial derivatives of the stress components $S_{zz}, S_{xz}, S_{xx}$. The CPML coefficient profiles $b_z, b_x, a_z, a_x, K_z, K_x$ are defined in (Martin et al., 2008), and $b_{zh}, b_{xh}, a_{zh}, a_{xh}, K_{zh}, K_{xh}$ are such coefficients shifted by half-grid due to the staggered-grid configuration. The coefficients $c_z, c_x$ are

the magnitudes of the normal stress components when implementing the borehole source. The density and shear modulus are averaged as follows:

1. $\rho_a$ is the density at the circles:

$$\rho_{a;i,j} = \frac{1}{2}(\rho_{i,j} + \rho_{i+1,j}) \tag{S32}$$

2. $\rho_b$ is the density at the boxes:

$$\rho_{b;i,j} = \frac{1}{2}(\rho_{i,j} + \rho_{i,j+1}) \tag{S33}$$

3. $\mu_{\text{ave}}$ is the shear modulus at the black dots:

$$\mu_{\text{ave};i,j} = 4/\left(\frac{1}{\mu_{\text{ave};i,j}} + \frac{1}{\mu_{\text{ave};i+1,j}} + \frac{1}{\mu_{\text{ave};i,j+1}} + \frac{1}{\mu_{\text{ave};i+1,j+1}}\right), \tag{S34}$$

and is set to zero when $\mu$ at any of the four corners is zero.

To derive the discrete adjoint system, we formulate the Lagrangian as

$$\begin{aligned}
\mathcal{L} =& \frac{1}{2}\sum_{r=1}^{N_r}\left[d_r^{t+1} - \left(c_z\mathcal{Q}_r(S_{zz}^{t+1}) + c_x\mathcal{Q}_r(S_{xx}^{t+1})\right)\right]^2 \\
&+ \left\langle \tilde{\varphi}_{zz}^{t+1}, \quad \varphi_{zz}^{t+1} - b_z\varphi_{zz}^{t} - a_z D_z^- V_z^t \right\rangle \\
&+ \left\langle \tilde{\varphi}_{xx}^{t+1}, \quad \varphi_{xx}^{t+1} - b_x\varphi_{xx}^{t} - a_x D_x^- V_x^t \right\rangle \\
&+ \left\langle \tilde{S}_{zz}^{t+1}, \quad S_{zz}^{t+1} - S_{zz}^{t} - (\lambda+2\mu)\left[\frac{1}{K_z}D_z^- V_z^t + \varphi_{zz}^{t+1}\right]\Delta t - \lambda\left[\frac{1}{K_x}D_x^- V_x^t + \varphi_{xx}^{t+1}\right]\Delta t - c_z f^t \Delta t \right\rangle \\
&+ \cdots \\
&+ \left\langle \tilde{V}_x^{t+1}, \quad V_x^{t+1} - V_x^t - \left[\frac{1}{K_z}D_z^- S_{xz}^{t+1} + \phi_{xz_z}^{t+1} + \frac{1}{K_{xh}}D_x^+ S_{xx}^{t+1} + \phi_{xx_x}^{t+1}\right]\frac{1}{\rho_b}\Delta t, \right\rangle
\end{aligned} \tag{S35}$$

where the variables with a tilde are the adjoint wavefield variables or the Lagrange multipliers, and the large bracket denotes discrete inner product in space and time, and $\mathcal{Q}$ is the sampling operator at receiver $r$.

Using the adjoint method, we obtain the adjoint equations

$$\tilde{V}_x^t - \tilde{V}_x^{t+1} + a_x D_x^+ \tilde{\varphi}_{xx}^{t+1} + \lambda \frac{1}{k_x} D_x^+ \tilde{S}_{zz}^{t+1} \Delta t + (\lambda + 2\mu) \frac{1}{k_x} D_x^+ \tilde{S}_{xx}^{t+1} \Delta t + a_{zh} D_z^- \tilde{\varphi}_{xz}^{t+1} + \mu_{\text{ave}} \frac{1}{k_{zh}} D_z^- \tilde{S}_{xz}^{t+1} \Delta t = 0$$

$$\tilde{\phi}_{xx\_x}^t - b_{xh} \tilde{\phi}_{xx\_x}^{t+1} - \tilde{V}_x^t \frac{1}{\rho_b} \Delta t = 0$$

$$\tilde{\phi}_{xz\_z}^t - b_z \tilde{\phi}_{xz\_z}^{t+1} - \tilde{V}_x^t \frac{1}{\rho_b} \Delta t = 0$$

$$\tilde{V}_z^t - \tilde{V}_z^{t+1} + a_z D_z^+ \tilde{\varphi}_{zz}^{t+1} + (\lambda + 2\mu) \frac{1}{k_z} D_z^+ \tilde{S}_{zz}^{t+1} \Delta t + \lambda \frac{1}{k_z} D_z^+ \tilde{S}_{xx}^{t+1} \Delta t + a_{xh} D_x^- \tilde{\varphi}_{zx}^{t+1} + \mu_{\text{ave}} \frac{1}{k_{xh}} D_x^- \tilde{S}_{xz}^{t+1} \Delta t = 0$$

$$\tilde{\phi}_{xz\_x}^t - b_x \tilde{\phi}_{xz\_x}^{t+1} - \tilde{V}_z^t \frac{1}{\rho_a} \Delta t = 0$$

$$\tilde{\phi}_{zz\_z}^t - b_{zh} \tilde{\phi}_{zz\_z}^{t+1} - \tilde{V}_z^t \frac{1}{\rho_a} \Delta t = 0$$

$$\tilde{S}_{xz}^t - \tilde{S}_{xz}^{t+1} + a_x D_x^+ \tilde{\phi}_{xz\_x}^t + \frac{1}{k_x \rho_a} D_x^+ \tilde{V}_z^t \Delta t + a_z D_z^+ \tilde{\phi}_{xz\_z}^t + \frac{1}{k_z \rho_b} D_z^+ \tilde{V}_x^t \Delta t = 0$$

$$\tilde{\varphi}_{zx}^t - b_{xh} \tilde{\varphi}_{zx}^{t+1} - \tilde{S}_{xz}^t \mu_{\text{ave}} \Delta t = 0$$

$$\tilde{\varphi}_{xz}^t - b_{zh} \tilde{\varphi}_{xz}^{t+1} - \tilde{S}_{xz}^t \mu_{\text{ave}} \Delta t = 0$$

$$\tilde{S}_{xx}^t - \tilde{S}_{xx}^{t+1} + a_{xh} D_x^- \tilde{\phi}_{xx\_x}^t + \frac{1}{k_{xh} \rho_b} D_x^- \tilde{V}_x^t \Delta t + c_x \left( c_z S_{zz}^t + c_x S_{xx}^t - d^t \right) = 0$$

$$\tilde{S}_{zz}^t - \tilde{S}_{zz}^{t+1} + a_{zh} D_z^- \tilde{\phi}_{zz\_z}^t + \frac{1}{k_{zh} \rho_a} D_z^- \tilde{V}_z^t \Delta t + c_z \left( c_z S_{zz}^t + c_x S_{xx}^t - d^t \right) = 0$$

$$\tilde{\varphi}_{xx}^t - b_x \tilde{\varphi}_{xx}^{t+1} - \lambda \tilde{S}_{zz}^t \Delta t - (\lambda + 2\mu) \tilde{S}_{xx}^t \Delta t = 0$$

$$\tilde{\varphi}_{zz}^t - b_z \tilde{\varphi}_{zz}^{t+1} - (\lambda + 2\mu) \tilde{S}_{zz}^t \Delta t - \lambda \tilde{S}_{xx}^t \Delta t = 0 \tag{S36}$$

Note that the system is solved backwards in time. For example, the gradient of the objective function with respect to $\lambda$ is

$$\nabla_J \lambda_{i,j} = -\sum_{t=1}^{N_t} \left( \tilde{S}_{zz;i,j}^{t+1} + \tilde{S}_{xx;i,j}^{t+1} \right) \left( D_z^- V_{z;i,j}^t + D_x^- V_{x;i,j}^t \right) \Delta t, \tag{S37}$$

72 where $N_t$ is the number of simulation steps.

## SI 5. An Example of Implementation of Customized PDE operators

We discuss the discretization and numerical implementation of forward modeling and gradient computation in this section. Since the discrete adjoint scheme for the elastic wave equation is discussed in 4, we mainly focus on the implementation of the forward and backward methods for operators of a single time step in the two-phase flow equations.

## SI 5.1. Forward Operation

In the forward simulations, we solve the discretized potential equation and saturation equation at each time step $n$:

$$-\nabla \cdot \Big( m_t \left( S_2^n \right) K \nabla \Psi_2^n \Big) = \nabla \cdot \Big( m_1 (S_2^n) K \nabla \Psi_c (S_2^n) \Big) + q^n, \tag{S38}$$

$$\phi(S_2^{n+1} - S_2^n) - \nabla \cdot \Big( m_2 (S_2^{n+1}) K \nabla \Psi_2^n \Big) \Delta t = \left( q_2^n + q_1^n \frac{m_2(S_2^{n+1})}{m_1(S_2^{n+1})} \right) \Delta t, \tag{S39}$$

where the upper script $n$ stands for time step $n$, and $\Delta t$ denotes the interval of a single time step. We first solve for $\Psi_2^n$ using $S_2^n$, and then we solve for $S_2^{n+1}$ with the obtained $\Psi_2^n$. In the saturation equation, we adopt the backward-Euler time scheme, which means that saturation-dependent parameters in the equation are functions of the to-be-solved saturation at time $n+1$ ($S_2^{n+1}$). This makes the time-stepping scheme implicit, which has the advantage that it is unconditionally stable, and thus the time step can be large.

In actual implementations, we divide the whole processes into four sequential forward operators:

$$m_1, m_t, \Psi_c = f_{\texttt{op1}}(S_2^n) \tag{S40}$$

$$\tilde{q}^n = f_{\texttt{op2}}(K, m_1, \Psi_c, q^n) \tag{S41}$$

$$\Psi_2^n = f_{\texttt{op3}}(K, m_t, \tilde{q}^n) \tag{S42}$$

$$S_2^{n+1} = f_{\texttt{op4}}(S_2^n, K, \Psi_2^n, \phi, q_2^n), \tag{S43}$$

where the $f_{\mathsf{op1}}$ computes mobilities $m_1, m_t$ and capillary potential $\Psi_c$ based on $S_2^n$, the $f_{\mathsf{op2}}$ computes the right-hand side of the discretized potential equation (S38):

$$\tilde{q}^n = \nabla \cdot \Big( m_1 K \nabla \Psi_c \Big) + q^n, \tag{S44}$$

the $f_{\mathsf{op3}}$ solves the Poisson equation from Eq. (S38):

$$-\nabla \cdot \Big( m_t K \nabla \Psi_2^n \Big) = \tilde{q}^n, \tag{S45}$$

and finally $f_{\mathsf{op4}}$ solves the non-linear implicit discretized saturation equation (S39) with the Newton-Raphson method (6).

For the spatial discretization, we adopt a second-order finite difference scheme in a cell-center grid, which is equivalent to the two-point-flux finite volume method (Lie, 2019). Fig. SI 3 shows the computational grid, where the saturation, potential, and other parameters are allocated in the center of the cells. The grid intervals $h$ of the cell in the $z$ and $x$ directions are the same, while in the $y$-direction perpendicular to the plane and the thickness of the cell is $h_y$.

The key to the spatial discretization of Eqs. (S38) and (S39) is the variable-coefficient Laplacian of the following form

$$\nabla \cdot \Big( m K \nabla \Psi \Big), \tag{S46}$$

where $m$ can be $m_1, m_2$ or $m_t$, and $\Psi$ can be $\Psi_2^n$ or $\Psi_c$.

The $z$ and $x$ components of $\nabla \Psi$ are defined on half grid points, since $\Psi_{i,j}$ are defined on cell centers. Therefore, we need to interpolate mobility $m$ and permeability $K$ onto half grid points. We use the harmonic average of permeabilities in the two adjacent cells

as the permeability at half grid points:

$$
\begin{aligned}
K_{i,j+\frac{1}{2}} &= \frac{K_{i,j}\,K_{i,j+1}}{K_{i,j}+K_{i,j+1}} \\
K_{i+\frac{1}{2},j} &= \frac{K_{i,j}\,K_{i+1,j}}{K_{i+1,j}+K_{i,j}}.
\end{aligned} \tag{S47}
$$

As for mobilities $m$, we adopt the upwind scheme:

$$
\begin{aligned}
m_{i,j+\frac{1}{2}} &= \begin{cases} m_{i,j}, & \text{if } \Psi_{i,j} \geq \Psi_{i,j+1} \\ m_{i,j+1}, & \text{if } \Psi_{i,j+1} > \Psi_{i,j} \end{cases} \\
m_{i+\frac{1}{2},j} &= \begin{cases} m_{i,j}, & \text{if } \Psi_{i,j} \geq \Psi_{i+1,j} \\ m_{i+1,j}, & \text{if } \Psi_{i+1,j} > \Psi_{i,j} \end{cases}
\end{aligned} \tag{S48}
$$

With these definitions, the discretized Laplacian is

$$
\begin{aligned}
\nabla \cdot \Big(m_t K \nabla \Psi_2^n\Big) = \Big[ & m_{i,j+\frac{1}{2}} K_{i,j+\frac{1}{2}} \left(\Psi_{i,j+1} - \Psi_{i,j}\right) \\
& - m_{i,j-\frac{1}{2}} K_{i,j-\frac{1}{2}} \left(\Psi_{i,j} - \Psi_{i,j-1}\right) \\
& + m_{i+\frac{1}{2},j} K_{i+\frac{1}{2},j} \left(\Psi_{i+1,j} - \Psi_{i,j}\right) \\
& - m_{i-1/2,j} K_{i-\frac{1}{2},j} \left(\Psi_{i,j} - \Psi_{i-1,j}\right) \Big] \frac{1}{\Delta h^2}
\end{aligned} \tag{S49}
$$

We implement the no-flow condition Eq. (S9) by imposing the following conditions:

$$
\begin{aligned}
&\Psi_{i,j+1} - \Psi_{i,j} = 0, \ \text{if } j = N_x, \\
&\Psi_{i,j} - \Psi_{i,j-1} = 0, \ \text{if } j = 1, \\
&\Psi_{i+1,j} - \Psi_{i,j} = 0, \ \text{if } i = N_z, \\
&\Psi_{i,j} - \Psi_{i-1,j} = 0, \ \text{if } i = 1,
\end{aligned} \tag{S50}
$$

Hence, we get large sparse linear systems from both the potential equation or the saturation equation, and we use an Algebraic Multi-grid Method (AMG) solver (AMGCL) (Demidov, 2017) to solve them.

## SI 5.2. Backward

Since $f_{\mathsf{op1}}$ and $f_{\mathsf{op2}}$ can be implemented with built-in operators in the AD framework, the backward operators $b_{\mathsf{op1}}$ and $b_{\mathsf{op2}}$ are automatically handled. The remaining two operators $f_{\mathsf{op3}}$ and $f_{\mathsf{op4}}$ are customized operators, so we need to implement the backward operators $b_{\mathsf{op3}}$ and $b_{\mathsf{op4}}$[1]:

$$\frac{\partial \mathcal{J}}{\partial \Psi_2^n}\frac{\partial f_{\mathsf{op3}}}{\partial K}, \frac{\partial \mathcal{J}}{\partial \Psi_2^n}\frac{\partial f_{\mathsf{op3}}}{\partial m_t}, \frac{\partial \mathcal{J}}{\partial \Psi_2^n}\frac{\partial f_{\mathsf{op3}}}{\partial \tilde{q}^n} = b_{\mathsf{op3}}\left(\frac{\partial \mathcal{J}}{\partial \Psi_2^n}, \Psi_2^n, K, m_t, \tilde{q}^n\right) \tag{S51}$$

$$\begin{aligned} &\frac{\partial \mathcal{J}}{\partial S_2^{n+1}}\frac{\partial f_{\mathsf{op4}}}{\partial S_2^n}, \frac{\partial \mathcal{J}}{\partial S_2^{n+1}}\frac{\partial f_{\mathsf{op4}}}{\partial K}, \frac{\partial \mathcal{J}}{\partial S_2^{n+1}}\frac{\partial f_{\mathsf{op4}}}{\partial \Psi_2^n} \\ &= b_{\mathsf{op4}}\left(\frac{\partial \mathcal{J}}{\partial S_2^{n+1}}, S_2^{n+1}, S_2^n, K, \Psi_2^n, \phi, q_2^n\right) \end{aligned} \tag{S52}$$

We demonstrate how to implement $\frac{\partial \mathcal{J}}{\partial S_2^{n+1}}\frac{\partial f_4}{\partial K}$ as example. The rest backward operators are implemented similarly. First, the PDE-constraint can be written as

$$\begin{aligned} &\mathcal{H}(S_2^{n+1}, S_2^n, \Psi_2^n, K) \\ &= \phi(S_2^{n+1} - S_2^n) - \nabla\cdot\left(m_2(S_2^{n+1})K\nabla\Psi_2^n\right)\Delta t - \left(q_2^n + q_1^n\frac{m_2(S_2^{n+1})}{m_1(S_2^{n+1})}\right)\Delta t = 0 \end{aligned} \tag{S53}$$

The discretization in both space and time is.

$$\begin{aligned} &\phi_{i,j}\left(S_{2;i,j}^{n+1} - S_{2;i,j}^n\right) - \Big[m_{2;i,j+\frac{1}{2}}K_{i,j+\frac{1}{2}}\left(\Psi_{2;i,j+1} - \Psi_{2;i,j}\right) - m_{2;i,j-\frac{1}{2}}K_{i,j-\frac{1}{2}}\left(\Psi_{2;i,j} - \Psi_{2;i,j-1}\right) \\ &+ m_{2;i+\frac{1}{2},j}K_{i+\frac{1}{2},j}\left(\Psi_{2;i+1,j} - \Psi_{2;i,j}\right) - m_{2;i-1/2,j}K_{i-\frac{1}{2},j}\left(\Psi_{2;i,j} - \Psi_{2;i-1,j}\right)\Big]\frac{\Delta t}{\Delta h^2} \\ &- \left(q_{2;i,j}^n + q_{1;i,j}^n\frac{m_{2;i,j}}{m_{1;i,j}}\right)\frac{\Delta t}{h^2 h_y} = 0. \end{aligned} \tag{S54}$$

The symbol $S_{2;i,j}^{n+1}$, for example, stands for saturation $S_2$ at time step $n$ and at the center of cell $i, j$. The mobilities at half grid points are computed with Eq. (S48), where $m_{1;i,j}$ and $m_{2;i,j}$ are functions of the unknown saturation $S_{2;i,j}^{n+1}$. At the boundaries, we insert the discrete boundary conditions (Eq. (S50)) in Eq. (S54).

According to the recipe in Section 3 on deriving backward operators in AD for implicit time-schemes:

1. We first follow Eq. (27) to construct a linear system

$$\mathcal{H}_{S_2^{n+1}}^T \boldsymbol{\lambda} = -\left(\frac{\partial \mathcal{J}}{\partial S_2^{n+1}}\right)^T, \tag{S55}$$

and solve for the Lagrange multiplier $\boldsymbol{\lambda}$. The left-hand side of the equation is also the transpose of the Jacobian matrix used in the Newton-Raphson method. We assemble the Jacobian matrix by taking the derivative of $\mathcal{H} = 0$ with respect to $S_2^{n+1}$ in Eq. (S54) (including the mobilities) for every $(i,j)$, and put each of the row vectors in the matrix according to the row-major sequence in $(i,j)$.

2. Assemble the Jacobian matrix of parameters. For example, to compute $\frac{\partial \mathcal{J}}{\partial S_2^{n+1}} \frac{\partial f_{\texttt{op4}}}{\partial K}$, we take the derivative of $\mathcal{H} = 0$ with respect to $K$ and assemble the matrix $\mathcal{H}_K$ in the same manner as in step 1.

3. Compute backward outputs. For example,

$$\frac{\partial \mathcal{J}}{\partial S_2^{n+1}} \frac{\partial f_{\texttt{op1}}}{\partial K} = \boldsymbol{\lambda}^T \mathcal{H}_K. \tag{S56}$$

## SI 6. The Newton-Raphson Method

We briefly outline the Newton-Raphson method to compute $S_2^{n+1}$ from $S_2^n$ for the non-linear saturation equation. First, we define the residual vector as

$$R(S) = \phi(S - S_2^n) - \nabla \cdot (m_2(S) K \nabla \Psi_2^n)\, \Delta t - q_2^n \Delta t. \tag{S57}$$

Using Taylor expansion, we have

$$R(S) = R(S_2^n) + R'(S_2^n)(S - S_2^n) + \mathcal{O}(\|S - S_2^n\|). \tag{S58}$$

Since the residual function equals zero vector at $S_2^{n+1}$, we attempt to find $S$ that satisfy this condition, and then arrive at

$$-R(S_2^n) = R'(S_2^n)\Delta S, \tag{S59}$$

where $R'(S_2^n)$ is the Jacobian matrix of $R$ with respect to $S_2$ at $S_2^n$. Solving sparse system, we obtain $\Delta S$ and make the update

$$S \leftarrow S + \alpha \Delta S, \tag{S60}$$

where $\alpha$ is the step length that is set as 1 initially. If the updated $S$ does not reduce the norm of the residual function, or it is not within the bounds of $[0, 1]$, we divide $\alpha$ by half ($\alpha = 0.5\alpha$) and update $S$ with the new $\alpha$ until those requirements are satisfied. This is the back-tracking line search for one Newton iteration. Then, we repeat the process until the convergence criterion is met: relative changes in the norm of the residual vectors are small than a given threshold. Hence, we find the saturation at time step $n + 1$.

## SI 7. Spatially Varying Permeability

We investigated a more challenging scenario where the permeability varies in the channel (Figure SI 4(a)). The permeability within the channel varies from 60 md to 180 md, and the permeability outside the channel is 20 md. The starting homogeneous model has the same permeability of 20 md as before. We adopted the same continuous inversion strategy as in section 4.4. We set the upper bound for permeability inversion as 190 md, and the lower bound 10 md. The inverted model is shown in Figure SI 4(b), where the low permeable section to the right of 450 m in the horizontal distance has been relatively well reconstructed, while the other low permeable section near the source on the left side is not. This error near the source could be the result of being trapped in a local minimum.

## SI 8. Seismic Sources and Receivers

We use a moment tensor source a approximate the radiation pattern of a piezoelectric source surrounded by fluid in a borehole. This model is based on an tensile crack

model (Aki & Richards, 2002). Therefore, both P and S waves are generated. Additionally, we use the same model for receivers to approximate a similar sensitivity pattern for hydrophones submerged in fluid in the borehole. The radiation/sensitivity pattern can be seen in Fig. SI 5.

## Notes

1. In this project, we write these parts in C++ according to the interface of TensorFlow, but the ADCME package can also take care of code written in other languages.

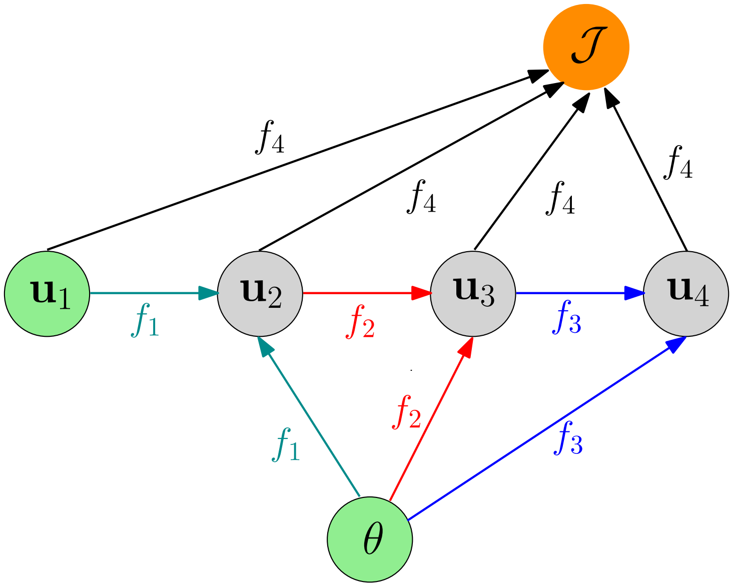


**Figure SI 1.** The computational graph of simplified slow-time process inversion. $\mathbf{u}_1$ and $\theta$ are the input vectors, $J$ is the output scalar, and $\mathbf{u}_2, \mathbf{u}_3,$ and $\mathbf{u}_4$ are intermediate variables.

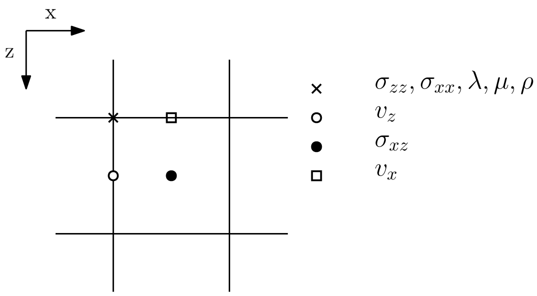


**Figure SI 2.** Cell $(i, j)$ of the staggered-grid for elastic wave equation. We define particle velocity components $v_z, v_x$, stress tensor components $\sigma_{zz}, \sigma_{xx}, \sigma_{xz}$ and elastic parameters $\lambda, \mu, \rho$ of spatial index $(i, j)$ in the annotated locations.

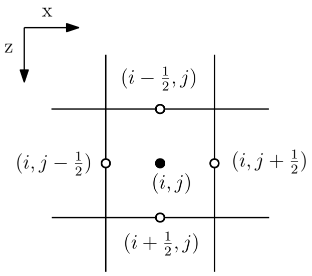


**Figure SI 3.** The cell-centered grid for two-phase flow equations. For cell $(i, j)$ shown in the figure, quantities are defined in the central black dot. We interpolate those quantities at the half grid points illustrated by circles for computation of second-order derivatives at the black dots. The grid intervals in the $z$ and $x$ directions are the same. The cell has a thickness of $h_y$.

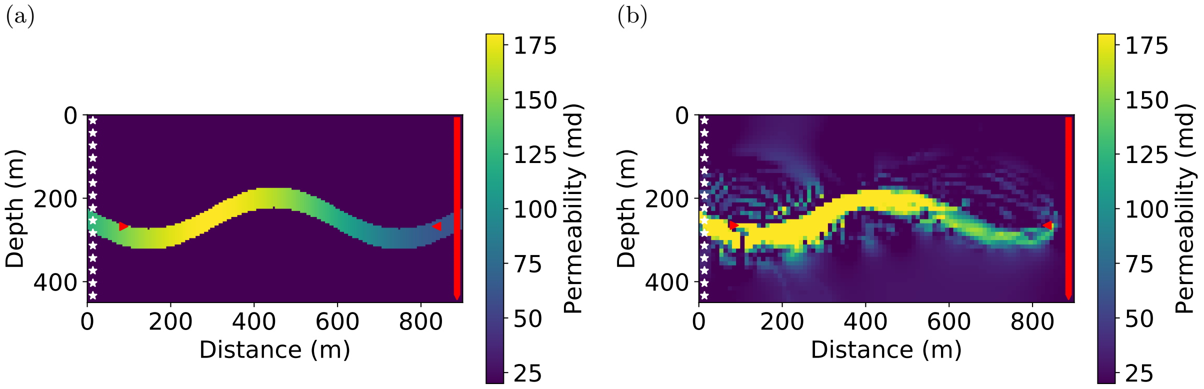


**Figure SI 4.** The inversion results of a channel model with spatially variable permeability. (a) The true permeability model; (b) the inverted permeability model with the continuous inversion strategy. The initial model is homogeneous with 20 md permeability as previous experiments.

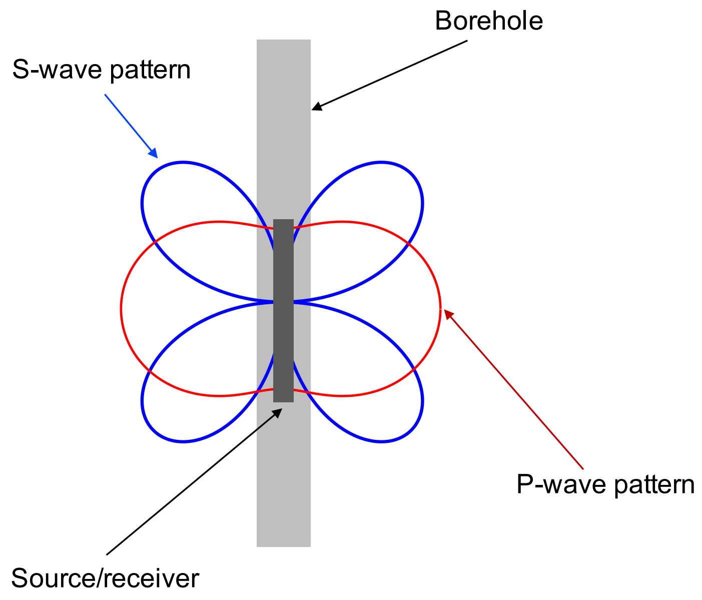


**Figure SI 5.** Radiation/sensitivity patterns (D. Li et al., 2019).

## References


Aki, K., & Richards, P. G. (2002). *Quantitative seismology* (Second ed.). University Science Books.

Brie, A., Pampuri, F., Marsala, A., Meazza, O., et al. (1995). Shear sonic interpretation in gas-bearing sands. In *Spe annual technical conference and exhibition.*

Demidov, D. (2017). Amgcl: An efficient, flexible, and extensible algebraic multigrid. *Lobachevskii Journal of Mathematics*, *40*, 535–546.

Li, D., Harris, J. M., Biondi, B., & Mukerji, T. (2019). *Seismic full waveform inversion : nonlocal similarity, sparse dictionary learning, and time-lapse inversion for subsurface flow* (Unpublished doctoral dissertation). Stanford University.

Li, R., Reynolds, A. C., Oliver, D. S., et al. (2001). History matching of three-phase flow production data. In *Spe reservoir simulation symposium.*

Lie, K.-A. (2019). *An introduction to reservoir simulation using matlab/gnu octave.* Cambridge University Press.

Marotzke, J., Giering, R., Zhang, K. Q., Stammer, D., Hill, C., & Lee, T. (1999). Construction of the adjoint mit ocean general circulation model and application to atlantic heat transport sensitivity. *Journal of Geophysical Research: Oceans*, *104*(C12), 29529–29547.

Martin, R., Komatitsch, D., & Ezziani, A. (2008). An unsplit convolutional perfectly matched layer improved at grazing incidence for seismic wave propagation in poroelastic media. *Geophysics*, *73*(4), T51–T61.

Mavko, G., Mukerji, T., & Dvorkin, J. (2009). *The rock physics handbook: Tools for seismic analysis of porous media.* Cambridge university press.

Oliver, D. S., & Chen, Y. (2011). Recent progress on reservoir history matching: a review.

*Computational Geosciences*, *15*(1), 185–221.

Wang, K.-Y., Lary, D., Shallcross, D., Hall, S., & Pyle, J. (2001). A review on the use of the adjoint method in four-dimensional atmospheric-chemistry data assimilation. *Quarterly Journal of the Royal Meteorological Society*, *127*(576), 2181–2204.
